# Supplementary material for: Exploiting Explicit Paths for Multi-hop Reading Comprehension
Source: arXiv:1811.01127 source file (2019-07-08)
Supplement: Supplementary file 1 [file appendix.tex]

\appendix
\section{Appendix}

% \todo{add some text. may be some more analysis? or examples of failure / success? or even one of those nice example figures from Souvik's talk?}

\begin{figure*}[tb]
\centering
\includegraphics[width=0.9\textwidth]{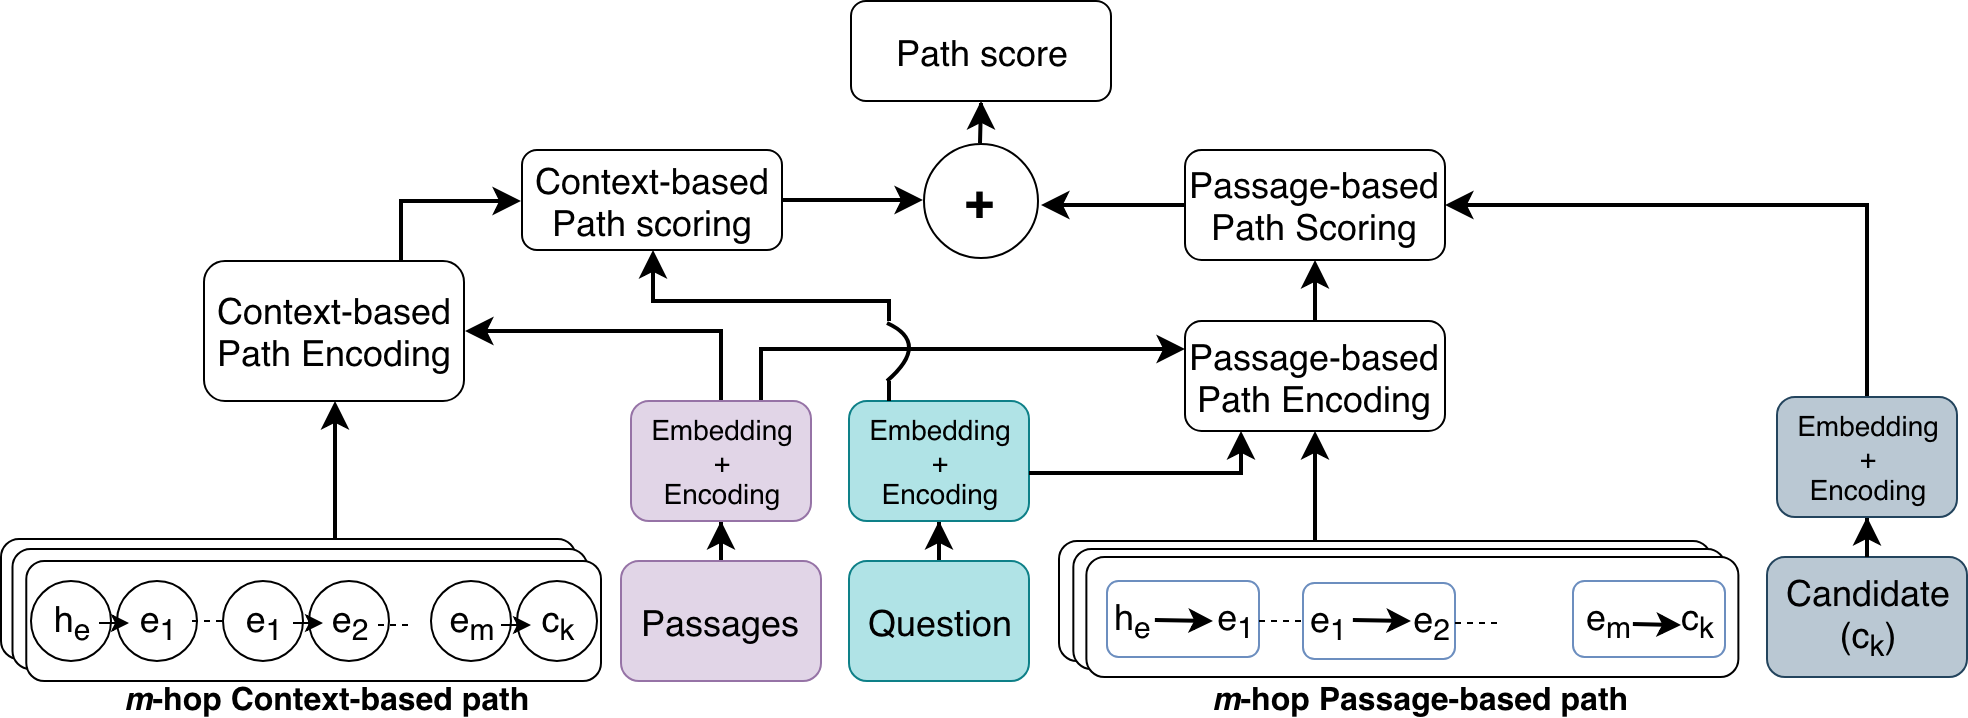}
\caption{Architecture of the path scoring module for $m$-hop paths.}
\label{fig:m_path_enc_diagram}
\end{figure*}

Figure \ref{fig:m_path_enc_diagram} depicts the path scoring module for a generic $m$-hop path. The overall architecture is similar with the 2-hop path scoring, except a recurrent network (LSTM, GRU etc.) needs to be used for path composition to tackle the variable number of hops.

%------%
\begin{table*}[tb]
\small
\centering
\begin{tabular}{|p{15cm}|}
\hline
\textbf{Question}: This can be used to light up a light \entA{bulb} \\
\textbf{Answer}: \entD{biofuel} \\
\textbf{Rank-1 Path}: (bulb, electricity, biofuel) \\
\underline{Passage1}: ... light \entA{bulbs} use \entB{electricity} ...\\
\underline{Passage2}: ... \entD{biofuel} is used to produce \entB{electricity} by burning ... \\
%------%
\textbf{Rank-2 Path}: (bulb, electricity, biofuel) \\
\underline{Passage1}: ... some light \entA{bulbs} convert \entB{electricity} into light and heat energy ...\\
\underline{Passage2}: ... \entD{biofuel} is used to produce \entB{electricity} by burning ... \\
\hline
%------------------%
\hline
\textbf{Question}: The circulatory system brings \entA{oxygen} to the \entA{body} from where ? \\
\textbf{Answer}: the \entD{chest} \\
\textbf{Rank-1 Path}: (oxygen, lung, chest) \\
\underline{Passage1}: ... the circulatory system brings \entA{oxygen} from the \entB{lungs} to the rest of the body ...\\
\underline{Passage2}: ... \entB{lungs} in \entD{chest} , part of the circulatory system ... \\
%-------%
\textbf{Rank-2 Path}: (body, part, chest) \\
\underline{Passage1}: ... Bones support all \entB{part}s of the \entA{body} and protect the brain and organs of the chest . ...\\
\underline{Passage2}: ... \entD{lungs} in chest , \entB{part} of the circulatory system ... \\
\hline
\end{tabular}
\caption{Two top-scoring paths for sample OpenBookQA Dev questions.}
\label{tab:extracted_paths_obqa}
\end{table*}
%-------------%

Table \ref{tab:extracted_paths_obqa} shows 2 top-ranked paths for examples taken from OpenBookQA development set where our proposed model could correctly predict the answer. As discussed in the paper, our proposed approach works by composing relation vectors between entities, and then combine to obtain a path representation.
For instance, the question is equivalent to {\em (bulb, can\_be\_used\_to\_light\_up, ?)}. 
Here, the rank-1 path is implicitly composing the relations {\em can\_be\_light\_up\_with}, i.e., {\em (bulbs, can\_be\_light\_up\_with, electricity)}, and {\em produced\_by}, i.e. {\em (electricity, produced\_by, biofuel)}.

%------%
\begin{table*}[tb]
\small
\centering
\begin{tabular}{|p{15cm}|}
\hline
\textbf{Reason of error}: ambiguous answer \\
\textbf{Question}: instance\_of \entA{singapore institute of management} \\
\textbf{Predicted Answer}: \entD{university} \\
\textbf{Reference Answer}: bussiness school \\
\textbf{Top Path}: (singapore institute of management, education, university) \\
\underline{Passage1}: ..The \entA{Singapore Institute of Management} ( abbreviation : SIM ; Chinese : ) is Singapore 's largest provider of private tertiary \entB{education} and professional training ...\\
\underline{Passage2}: ... Autonomous \entD{university} typically refers to a university ... or government agency regulating higher \entB{education} ... \\
%------------------%
\hline
\textbf{Reason of error}: ambiguous answer \\
\textbf{Question}: headquarters\_location \entA{london travelwatch} \\
\textbf{Predicted Answer}: \entD{westminster} \\
\textbf{Reference Answer}: city of london \\
\textbf{Top Path}: (london travelwatch, transport for london, westminster) \\
\underline{Passage1}: ... \entA{London TravelWatch} is a statutory ... It is the transport watchdog for services provided by \entB{Transport for London} , which includes ...\\
\underline{Passage2}: ... \entB{Transport for London} ( TfL ) is a local government body responsible for the ... Its head office is in Windsor House in the City of \entD{Westminster} ... \\
%------------------%
\hline
\end{tabular}
\caption{Sample multi-hop questions from \wikihop development set where our system failed to predict correctly.}
\label{tab:error_wikihop}
\end{table*}
%-------------%

%------%
\begin{table*}[tb]
\small
\centering
\begin{tabular}{|p{15cm}|}
\hline
\textbf{Reason of error}: meaningless entity linking \\
\textbf{Question}: An example of lots kinetic \entA{energy} would be \\
\textbf{Predicted Answer}: sitting without \entD{moving} anywhere \\
\textbf{Reference Answer}: An aircraft taking a trip \\
\textbf{Top Path}: (energy, object, move) \\
\underline{Passage1}: \entB{Objects} have kinetic \entA{energy} because they are moving .\\
\underline{Passage2}: ... as an \entB{object} \entD{moves} , the kinetic energy of that object will increase ... \\
%------------------%
\hline
\textbf{Reason of error}: irrelevant retrieved sentences \\
\textbf{Question}: Stopped means \entA{lack} of what ? \\
\textbf{Predicted Answer}: \entD{warmth} \\
\textbf{Reference Answer}: velocity \\
\textbf{Top Path}: (lack, plant, warmth) \\
\underline{Passage1}: Bryophytes are non - vasular \entA{plants} , meaning they \entA{lack} xylem and phloem , which are found in higher plants \\
\underline{Passage2}: \entB{Plants} grow in clumps to conserve \entD{warmth} \\
%------------------%
\hline
\end{tabular}
\caption{Sample multi-hop questions from OpenBookQA development set where our system failed to predict correctly.}
\label{tab:error_obqa}
\end{table*}
%-------------%

Table \ref{tab:error_wikihop} and \ref{tab:error_obqa} shows some samples from \wikihop and OpenBookQA development set respectively, where our system incorrectly predicted the answer.
